# Supplementary material for: How Do Mobile Applications Enhance Security? An Exploratory Analysis of Use Cases and Provided Information
Source: arXiv:2504.14421 source file (2025-04-19)
Supplement: Supplementary file 1 [file A-first.tex]

\section{First Appendix}
\label{app:first}
\noindent
Remember not to indent in the Appendix as well. You can also have sub-appendices.

\subsection{First subappendix}
\label{sapp:tables}
\noindent
Appendices are useful to report tables or figures that cannot be put in the main text.
